# Supplementary material for: From Obstacles to Resources: Semi-supervised Learning Faces Synthetic Data Contamination
Source: arXiv:2405.16930 source file (2024-11-27)
Supplement: Supplementary file 1 [file X_suppl.tex]

\clearpage
\setcounter{page}{1}
\maketitlesupplementary

We provide additional analysis and implementation details of constructing the RS-SSL benchmark and training the models. We also provide our code. Our code and synthetic data will be made public upon acceptance.

\begin{figure}[t]
  \centering
  \includegraphics[width=0.99\linewidth]{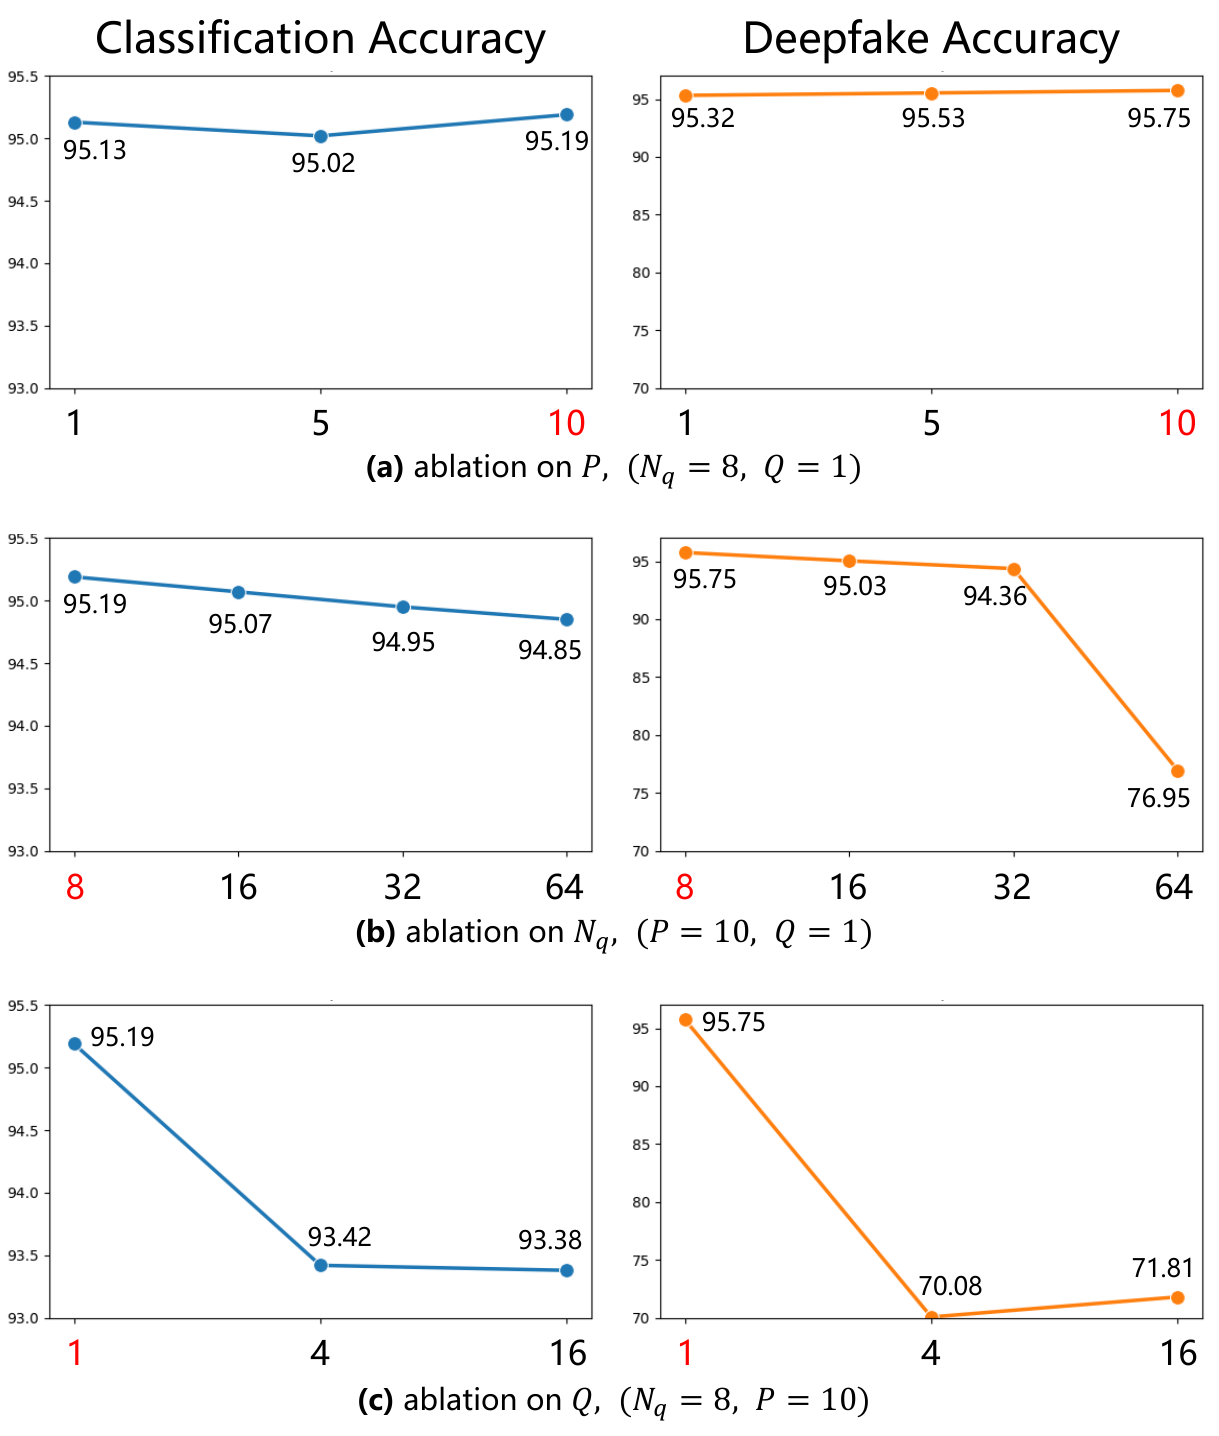}
  \caption{Ablation studies on CSQueue hyper-parameters $N_{q}$, $P$, and $Q$. We use CIFAR-10~\cite{krizhevsky2009learning} with 25 labeled images per class and synthetic ratio $\alpha=0.5$. The red values are our final settings.}
  \label{fig_sup_2}
\end{figure}

\section{Additional analysis}
\subsection{Ablations on CSQueue}
We conduct ablation studies on the hyper-parameters ($N_{q}$, $P$, and $Q$) of our CSQueue. Fig.~\ref{fig_sup_2} demonstrates the accuracy curves of the classifier and the deepfake detector. The results show that RSMatch is relatively robust to the selected queue number $P$. Meanwhile, a larger queue size $N_{q}$ will not bring benefits as shown in Fig.~\ref{fig_sup_2} (b), as the noisy sample in the queue will not be dropped quickly. Moreover, updating too many samples for one class (\ie, $Q$) in Fig.~\ref{fig_sup_2} (c) will also affect the performance, as noisy samples will more likely to be selected with the enqueued number increasing.

\subsection{Deepfake detection accuracy}

\begin{table}[t]
\centering
\begin{center}
\resizebox{\linewidth}{!}{
\begin{tabular}{l|ccc}
\toprule
Dataset & \multicolumn{3}{c}{CIFAR-10} \\
\midrule
Synthetic ratio ($\alpha$) & 0.3 & 0.5 & 1.0 \\
\midrule
Ours-FixMatch &  92.45\scalebox{0.8}{$\pm$1.7} & 97.28\scalebox{0.8}{$\pm$2.6} & 97.53\scalebox{0.8}{$\pm$0.8} \\
Ours-FlexMatch &  92.05\scalebox{0.8}{$\pm$0.8} & 92.82\scalebox{0.8}{$\pm$0.4} & 85.93\scalebox{0.8}{$\pm$2.1} \\
Ours-SoftMatch &  94.30\scalebox{0.8}{$\pm$1.1} & 96.42\scalebox{0.8}{$\pm$0.3} & 87.51\scalebox{0.8}{$\pm$0.7} \\
\bottomrule
\end{tabular}
}

\vspace{10pt}

\resizebox{\linewidth}{!}{
\vspace{20pt}
\begin{tabular}{l|ccc}
\toprule
Dataset & \multicolumn{3}{c}{CIFAR-100} \\
\midrule
Synthetic ratio ($\alpha$) & 0.3 & 0.5 & 1.0 \\
\midrule
Ours-FixMatch &  90.27\scalebox{0.8}{$\pm$1.5} & 93.79\scalebox{0.8}{$\pm$0.2} & 96.74\scalebox{0.8}{$\pm$1.5} \\
Ours-FlexMatch &  90.93\scalebox{0.8}{$\pm$1.4} & 94.15\scalebox{0.8}{$\pm$0.6} & 94.28\scalebox{0.8}{$\pm$0.3} \\
Ours-SoftMatch &  85.93\scalebox{0.8}{$\pm$3.3} & 88.94\scalebox{0.8}{$\pm$0.8} & 95.97\scalebox{0.8}{$\pm$1.6} \\
\bottomrule
\end{tabular}
}

\vspace{10pt}

\resizebox{\linewidth}{!}{
\begin{tabular}{l|ccc|c}
\toprule
Dataset & \multicolumn{3}{c|}{TinyImageNet} & ImageNet\\
\midrule
Synthetic ratio ($\alpha$) & 0.3 & 0.5 & 1.0 & 0.5 \\
\midrule
Ours-FixMatch &  94.44\scalebox{0.8}{$\pm$2.7} & 94.79\scalebox{0.8}{$\pm$1.4} & 97.97\scalebox{0.8}{$\pm$1.2} & 96.87\scalebox{0.8}{$\pm$2.0} \\
\bottomrule
\end{tabular}
}
\end{center}
\caption{Deepfake detection accuracy (\%) with various synthetic ratios $\alpha$ on CIFAR-10~\cite{krizhevsky2009learning}, CIFAR-100~\cite{krizhevsky2009learning} with 25 labels per class and TinyImageNet~\cite{deng2009imagenet}, ImageNet~\cite{deng2009imagenet} with 10\% labels per class.}
\label{tab:tab_sup_2}
\end{table}
Table~\ref{tab:tab_sup_2} shows the accuracy of the deepfake detector in Table~1 and 3 of our original paper. The accuracy is evaluated on the unlabeled dataset. The results show that our method can effectively identify unlabeled synthetic images under the condition that no synthetic image labels are provided.

\section{Implementation details}

\subsection{RS-SSL benchmark}

We construct the RS-SSL benchmark by generating synthetic images and adding them to the unlabeled data of original SSL datasets. Take the CIFAR-10 dataset for example, we use the following steps to construct the benchmark.

\noindent\textbf{Prompts.} We feed the ten class names of the CIFAR-10 dataset into the pre-trained T5~\cite{raffel2020exploring} model to generate text prompts. We generate $M=200$ prompts for each class.

\begin{figure*}[t]
  \centering
  \includegraphics[width=0.99\linewidth]{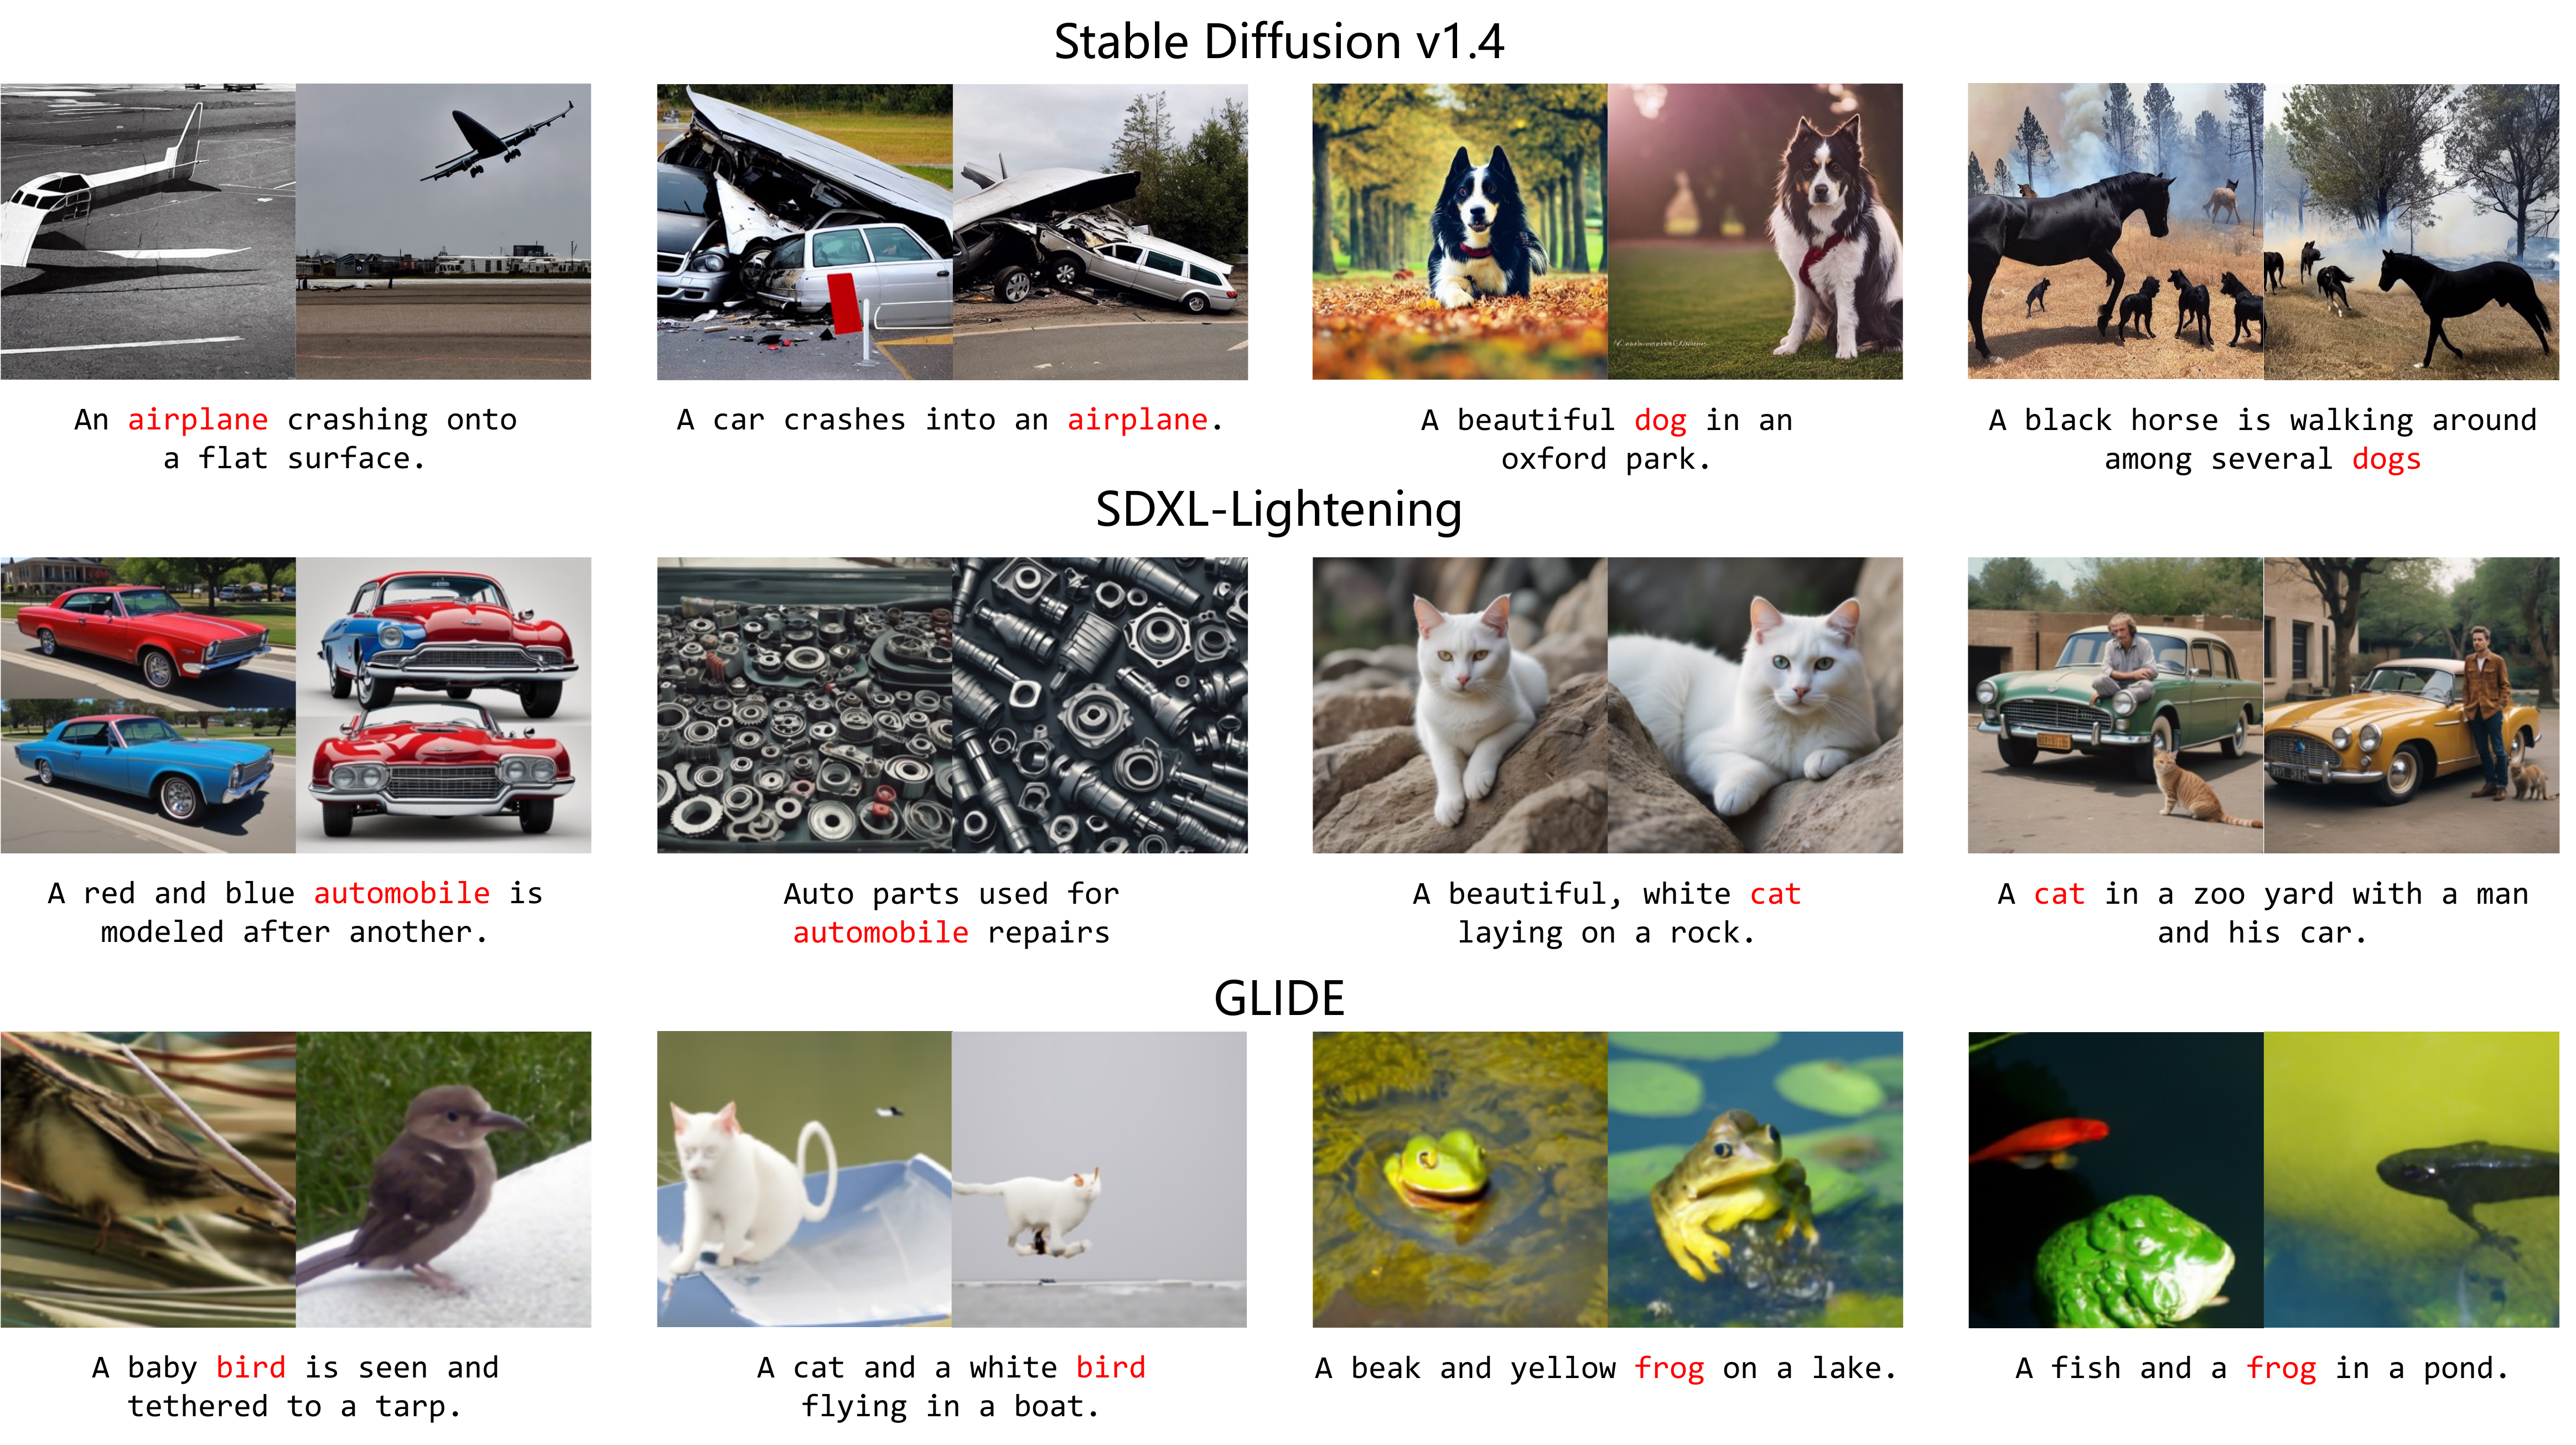}
  \caption{The synthetic images from three generative models with the prompts for CIFAR-10. Besides the images matching the target class, there are also images with noise and semantic bias. The grammatical errors in the prompts are caused by the T5 model. The red words are the target classes.}
  \label{fig_sup_1}
\end{figure*}
\begin{table*}[t]
\centering
\begin{center}
\resizebox{\linewidth}{!}{
\begin{tabular}{l|c|c|c|c|c|c}
\toprule
& Hyper-parameter & Description  & CIFAR-10 & CIFAR100 & TinyImageNet & ImageNet \\
\midrule
\multirow{9}{*}{\rotatebox{90}{SSL~(FixMatch)}} & $\tau$ & SSL confidence threshold & \multicolumn{4}{c}{0.95} \\
 & $\lambda$ & Unsupervised loss weight & \multicolumn{4}{c}{1} \\
 & $\beta$ & Momentum & \multicolumn{4}{c}{0.9} \\
 & $\alpha$ & EMA weight & \multicolumn{4}{c}{0.999} \\
 & $lr$ & Learning rate & \multicolumn{4}{c}{0.03} \\
 & $B$ & Labeled data batch size & \multicolumn{4}{c}{64} \\
 & Iteration & Training iterations & \multicolumn{4}{c}{$2^{20}$} \\
 \cmidrule{2-7}
& $\mu$ & Unlabeled data batch ratio & 7 & 7 & 7 & 1 \\
 & Weight decay & Weight decay & 0.0005 & 0.001 & 0.0005 & 0.0001\\
\midrule
\multirow{3}{*}{\rotatebox{90}{Ours}} & $N_q$ & The sub-queue size of CSQueue  & \multicolumn{4}{c}{8} \\
 & $P$ & The selected sub-queue number for each iteration  & \multicolumn{4}{c}{10} \\
 & $Q$ & The enqueued number for each iteration  & \multicolumn{4}{c}{1} \\
 \bottomrule
\end{tabular}
}
\end{center}
\caption{Hyper-parameters of RSMatch with FixMatch as the basic SSL method.}
\label{tab:tab_sup_1}
\end{table*}

\noindent\textbf{Image generation.} We use GLIDE~\cite{nichol2022glide}, Stable Diffusion v1.4 (SD14)~\cite{rombach2022high}, and SDXL-Lightening~\cite{lin2024sdxl} to generate images using the abovementioned prompts. For each class, we generate the same number of images with the original CIFAR-10 training dataset, \ie, 5,000 images. Thus, we generate $\lceil\frac{5000}{200\times3}\rceil = 9$ images with each generative model using each prompt. We use the diffusers~\cite{von-platen-etal-2022-diffusers} library for generation and follow the default settings of each model (\eg, scheduler, sampling steps, resolution, \etc). Fig.~\ref{fig_sup_1} demonstrates some generated results. After generation, we resize the images into the size of CIFAR-10, \ie, $32\times32$.

\noindent\textbf{Benchmark construction.} For each class, we randomly select synthetic images and add them to the original CIFAR-10 dataset to construct the benchmark. For example, given \textit{synthetic ratio} $\alpha=0.5$, we randomly select $\lceil5000\times0.5\rceil = 2500$ images from our generated samples. Thus, the final dataset will consist of 7,500 images per class. Finally, following previous SSL methods, we randomly select labeled images from the real data, and the remaining images are unlabeled data.

% \textbf{Our synthetic images.} We demonstrate some generated images with the prompts in Figure~\ref{fig_sup_1}. Note that these images will resize to the size of the target real dataset during training.

\subsection{Training details}

\noindent\textbf{Environment.} All experiments are conducted on one NVIDIA A100 GPU with 40GB memory. We use Python 3.8, PyTorch~\cite{paszke2017automatic} 2.1.2 with CUDA 12.2. All the methods are implemented using the SSL codebase USB~\cite{wang2022usb}. Following the codebase's setting and previous methods~\cite{zhang2021flexmatch, li2023iomatch}, we report the accuracy of the best checkpoint during training for all the experiments.

\noindent\textbf{Hyper-parameters.} Our RS-Match applies different SSL methods as the basic framework. Thus, we directly use their settings for SSL. Table~\ref {tab:tab_sup_1} summarizes the hyper-parameters using FixMatch as the basic SSL method. For the optimizer, we use SGD with the cosine learning rate decay. For other basic SSL methods and the rivals in our paper, we use their original settings for fair comparison. 

% \section{Rationale}
% \label{sec:rationale}
% % 
% Having the supplementary compiled together with the main paper means that:
% % 
% \begin{itemize}
% \item The supplementary can back-reference sections of the main paper, for example, we can refer to \cref{sec:intro};
% \item The main paper can forward reference sub-sections within the supplementary explicitly (e.g. referring to a particular experiment); 
% \item When submitted to arXiv, the supplementary will already included at the end of the paper.
% \end{itemize}
% % 
% To split the supplementary pages from the main paper, you can use \href{https://support.apple.com/en-ca/guide/preview/prvw11793/mac#:~:text=Delete%20a%20page%20from%20a,or%20choose%20Edit%20%3E%20Delete).}{Preview (on macOS)}, \href{https://www.adobe.com/acrobat/how-to/delete-pages-from-pdf.html#:~:text=Choose%20%E2%80%9CTools%E2%80%9D%20%3E%20%E2%80%9COrganize,or%20pages%20from%20the%20file.}{Adobe Acrobat} (on all OSs), as well as \href{https://superuser.com/questions/517986/is-it-possible-to-delete-some-pages-of-a-pdf-document}{command line tools}.
